# Supplementary material for: Students' Perceptions and Preferences of Generative Artificial Intelligence Feedback for Programming
Source: arXiv:2312.11567 source file (2023-12-17)
Supplement: Supplementary file 1 [file Appendix.pdf]

# Appendix A

| Comparison | Feedback with Prompt That Includes Student's Code | Feedback with Prompt that doesn't include student's code |
|---|---|---|
| 2<br>Similar advice | Dear student, I hope this message finds you well. I have reviewed your Java code for Lab 6 Math Calculations and I have some feedback for you. Firstly, I appreciate your effort in completing the assignment. However, I noticed that your code did not pass all the test cases. Specifically, the median calculation for four integers is not correct.<br><br>To improve your code, I suggest you review the median calculation for four integers. You can use the formula provided in the comments of the method to calculate the median. Additionally, I recommend that you review the checkstyle errors in your code.<br><br>Overall, I believe that with some improvements, you can excel in future homework. Keep up the good work and don't hesitate to reach out if you have any questions. | Dear student, I hope this message finds you well. I wanted to provide you with some feedback on your recent Java homework, Lab 6 Math Calculations.<br>Firstly, I want to commend you on your efforts and hard work. It's clear that you put in a lot of effort into your code, and that's a great attitude to have.<br>However, I noticed that your code did not pass all the test cases. Specifically, the median calculation was incorrect. I recommend reviewing your code and checking your calculations to ensure that you are getting the correct result.<br>Additionally, I noticed that your code had some Checkstyle errors. Please take some time to review the Checkstyle guidelines and ensure that your code adheres to them.<br>Overall, I believe that with some additional practice and attention to detail, you can excel in future homework assignments. Keep up the good work and don't hesitate to reach out if you have any questions or concerns. |
| 3<br>Comprehensiveness | Dear student, Great job on completing your Java homework! I have reviewed your code and would like to provide you with some feedback to help you improve.<br><br>Firstly, your implementation of the \`isPalindrome\` method looks good. You correctly handle the case where the input array is null and throw an \`IllegalArgumentException\`. However, **I noticed that you are using the \`==\`** operator to compare strings. Remember that when comparing strings, you should use the \`equals\` method instead. So, make sure to update your code accordingly.<br><br>Secondly, your implementation of the \`equals2D\` method also looks good. You correctly handle the case where either of the input arrays is null and throw an \`IllegalArgumentException\`. However, **I noticed that you are using the \`Arrays.equals\`** method to compare arrays. This method compares the references of the arrays, not the actual contents. To compare the contents of the arrays, you should use nested loops to iterate over the elements and compare them individually.<br><br>Overall, your code is well-structured and easy to read. Keep up the good work! If you have any questions or need further clarification, feel free to ask. Keep practicing and you'll continue to improve | Dear student, Great job on completing Lab 12! You have shown a good understanding of the concepts and have successfully passed all of your unit and integration tests. Well done!<br><br>I noticed that you included the Arrays class methods in your code, which is not allowed. Remember to only use the methods and techniques that we have covered in class. Make sure to review the lab instructions and remove any unnecessary code.<br><br>Additionally, there were some checkstyle errors in your code. Take some time to go through the checkstyle rules and make the necessary adjustments to ensure your code follows the required style guidelines.<br><br>In terms of test coverage, your unit and integration tests for the isPalindrome() and equals2D() methods have good branch and line coverage. Keep up the good work in writing comprehensive tests to ensure the correctness of your code.<br><br>Overall, you have done a great job on this lab. Keep practicing and reviewing the concepts we have covered, and I'm confident that you will continue to excel in future assignments. |
| 4<br>Confusing information | Dear student, Great job on completing Lab 9! Your code is passing all of the unit and integration tests, which is a great accomplishment. However, there are a few things that you can improve on to make your code even better.<br><br>Firstly, **your code is missing Javadoc comments for the class and methods.** Adding these comments will help others understand your code better and make it easier to maintain in the future.<br><br>Secondly, your getInteger() method can be simplified. Instead of using a boolean variable to control the while loop, you can use a do-while loop to ensure that the user inputs a positive integer. This will make your code more concise and easier to read.<br><br>Lastly, your getSeries() method can **be improved by using a StringBuilder** instead of a String to concatenate the squares. This will make your code more efficient and reduce the amount of memory used.<br><br>Keep up the good work and don't hesitate to reach out if you have any questions or need further assistance. | Dear student, I hope this feedback finds you well. I have reviewed your Java homework submission for Lab 9: Series of Numbers. While you have passed all of your unit and integration tests, there are a few areas where you can improve.<br><br>Firstly, congratulations on including a .gitignore file and passing all of your tests. Your code also meets the checkstyle requirements, which is great to see.<br><br>However, I noticed that your code could benefit from more descriptive variable names. This will make your code easier to read and understand for others. Additionally, you could consider adding comments to explain the purpose of certain sections of your code.<br><br>In terms of your test coverage, you have good coverage for both the getInteger() and getSeries() methods. However, there is still room for improvement. You could consider adding more test cases to cover edge cases and ensure that your code is robust.<br><br>Overall, you have done a good job on this assignment. Keep up the good work and continue to strive for excellence in your future homework submissions. |

# Appendix B

| Guideline | Survey Questions |
|---|---|
| Present elaborated feedback in manageable units. | Was the feedback presented in small and manageable pieces to avoid overwhelming you? |
| Be specific and clear with feedback messages. (1) | Was the feedback specific and clear enough to be useful for the assignment? |
| Be specific and clear with feedback messages. (2) | Was the feedback tailored to your response rather than being a general comment applicable to the entire class? |
| Keep feedback as simple as possible but no simpler (based on learner needs and instructional constraints). | Was the feedback content simple enough to understand? |
| Reduce uncertainty between performance and goals. | Was the feedback clear enough to help you understand how well you performed and what you need to do in order to attain the goal of this lab assignment? |
| Give unbiased, objective feedback, written or via computer. | Do you perceive AI-generated feedback as unbiased and objective feedback? |
| Promote a “learning” goal orientation via feedback. | To what extent did the feedback highlight the importance of learning instead of your academic performance in the lab? (e.g. 1. Did the feedback highlight the importance of effort in enhancing learning and performance? 2. Did the feedback underscore the role of mistakes in the learning process? 3. Did the feedback motivate you to prioritize the process of learning?) |
| Avoid using “praise” sparingly, if at all. | Would you categorize the conveyed sentiment as positive, neutral, or negative? |
| Focus feedback on the task, not the learner. | N/A |
| Provide elaborate feedback to enhance learning. | N/A |
| Provide feedback after attempts. | N/A |

# Appendix C-1

| Label | Definition |
|---|---|
| Specific | AI is specific to the reason student fail |
| Simple/understandable/readability/clarity | AI is clear/simple to read |
| Motivational support | AI encourages students to move forward/engage |
| Wrong AI feedback | AI can be incorrect sometimes |
| more corrective suggestions | AI explains how to fix the bug |
| AI suggests alternative solutions | AI gives alternative solutions even if students are correct |
| Comprehensive | AI gives comprehensive feedback that covers wide. |
| no difference | Whether giving or not giving code to ChatGPT does not make a difference for students |
| Well Structured | AI feedback is well-structured, with clear organization in paragraphs |
| Original auto-feedback is confusing | Original feedback is confusing |

# Appendix C-2

| Label | Definition |
|---|---|
| Specific to test case | AI feedback explains which test cases are wrong and why they are wrong. |
| Specific to code | AI feedback is specific to the student's code and show root cause of issues in the student's code |
| External Resources | AI provide external resources to help students correct issues or further improve themselves |
| Align with lab instruction | AI feedback aligns with the assignment instructions on Moodle |
| More cristism | AI gives excessively positive feedback |
| Show example correct code | AI provides correct assignemnt code or code of similar problem |
| Concise/ simple/ clearity | The content of AI feedback is not redundant or wordy |
| Visualization/Structure | AI feedback is well-structured and visually appealing |
| good enough | AI feedback is good enough. |
| more corrective suggestions | AI provides more feedback on how to fix issues |
| additional help | AI provides feedback on additional topics that are out of scope of the assignment feedback such as java style and checkstyle |
| Alternative solutions | AI discusses alternative solutions to assignment problem |
| more personalized | AI feedback should be more personalized |
| More human-like sentences | AI should generate more human-like sentences in the feedback |
| More positive support | AI should provide more positive and encouraging feedback |
| AI educational support | Students want to learn more about AI tools and how the AI feedback is generated |
| Timely feedback | Students prefer timely feedback |
